# Supplementary material for: Ray-tracing image simulations of transparent objects with complex shape and inhomogeneous refractive index
Source: arXiv:2507.23145 source file (2026-04-21)
Supplement: Supplementary file 1 [file Kalita_RayTraceImageSims_SuppMat_arXiv.pdf]

## SUPPLEMENTAL MATERIAL

### Ray-tracing image simulations of transparent objects with complex shape and inhomogeneous refractive index

Armin Kalita,<sup>1</sup> Bryan Oller,<sup>1</sup> Thomas Paula,<sup>2</sup> Alexander Bußmann,<sup>2</sup> Sebastian Marte,<sup>1</sup> Gabriel Blaj,<sup>3</sup> Raymond G. Sierra,<sup>4</sup> Sandra Mous,<sup>4</sup> Kirk A. Larsen,<sup>4</sup> Xinxin Cheng,<sup>4</sup> Matt J. Hayes,<sup>4</sup> Kelsey Banta,<sup>4</sup> Stella Lisova,<sup>4</sup> Peter Nguyen,<sup>4</sup> Serge A. H. Guillet,<sup>4</sup> Divya Thanasekaran,<sup>4</sup> Silke Nelson,<sup>4</sup> Mengning Liang,<sup>4</sup> Stefan Adami,<sup>2</sup> Nikolaus A. Adams<sup>2</sup> and Claudiu A. Stan<sup>1,\*</sup>

<sup>1</sup>*Department of Physics, Rutgers University-Newark, Newark, NJ 07102, USA*

<sup>2</sup>*Chair of Aerodynamics and Fluid Mechanics, TUM School of Engineering and Design, Technical University of Munich, 85748 Garching bei München, Germany*

<sup>3</sup>*Technology Innovation Directorate, SLAC National Accelerator Laboratory, Menlo Park, CA 94025, USA*

<sup>4</sup>*Linac Coherent Light Source, SLAC National Accelerator Laboratory, Menlo Park, CA 94025, USA*

*\*email: claudiu.stan@rutgers.edu*

#### TABLE OF CONTENTS

|                                                                    |    |
|--------------------------------------------------------------------|----|
| 1. The ray-tracing model                                           | 2  |
| 2. Ray-tracing model testing and characterization                  | 5  |
| 3. Computation times                                               | 7  |
| 4. Focus scans and triple droplet merging                          | 7  |
| 5. The X-ray laser ablation of water drops                         | 11 |
| 6. Sensitivity, accuracy, and impact on fluid dynamics simulations | 15 |
| 7. Supplementary movies                                            | 19 |
| 8. Image processing                                                | 20 |
| 9. References                                                      | 21 |

# 1. The ray-tracing model

## 1.1 The light field illumination source

The purpose of the illumination source in the ray-tracing model is to replicate as closely as possible the experimental illumination. Ideally, this involves replicating, at every point in the object plane, the intensity and the angular distribution of the rays (*i.e.*, replicating the light field [14]). For our experiments this was unnecessary, because the angular distribution of rays had only small variations within a few hundred microns from where the drops are imaged. Also, for computational efficiency, the illuminated region in the model should be restricted to the vicinity of the drop. Therefore, we assumed the same angular distribution of rays from all points in the object plane, and we collected the properties of the experimental illumination using a single calibration step.

Figure S1 illustrates the experimental calibration and the generation of the virtual light field source (LFS). The LFS was built by tracing rays between two surfaces. The first surface is an image of a 200  $\mu\text{m}$  square pinhole, placed in the object plane at the location of the drops. The second surface is the image of the light cone emerging from the pinhole, imaged directly on the sensor of our camera, 10–20 mm downstream of the pinhole. We corrected the light cone image for the angular efficiency of the camera. This corrected light cone image does not provide a perfect measurement of the angular distribution of rays, because it is blurred due to the finite size of the pinhole and due to diffraction. Nevertheless, these effects spread the light from a point source to a spot on the order of 100  $\mu\text{m}$ , which is small compared to the approximately 10 mm diameter of the light cone image.

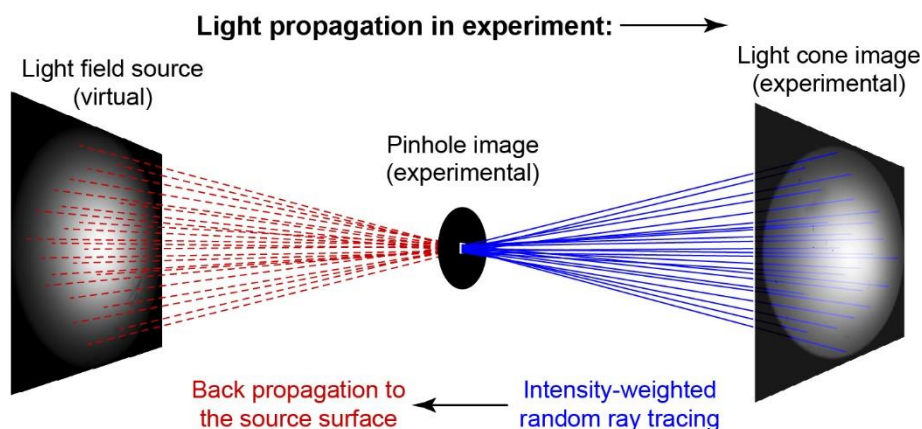

**Figure S1.** Generation of the light field source. A pinhole is placed in the object plane and imaged with the microscope, then the light cone from the pinhole is imaged on a camera sensor. Rays are traced between the pinhole and the image of the light cone, then back propagated to the surface of the virtual source, where their location and direction are computed and stored for use in the ray tracing model.

Rays were generated by connecting pixels from the two surfaces, and then back-propagated to the illumination source, where the ray intercept points and their angles were recorded. The pixels from the two surfaces were chosen randomly with weights proportional to the light intensity in the pixels. For the simulated images shown here,  $10^8$ – $10^9$  source rays were traced and written in a library that represents the virtual light field source. The rays were calculated using MATLAB (version 2021A and later) and written in a binary file using the light source format used by Zemax OpticStudio, which specified for each ray the x, y, and z coordinates, and the three direction cosines.

### 1.2 The model of the microscope objective

The objective lens we used (Mitutoyo M Plan Apo 20×) has a working distance  $WD = 20$  mm, which exceeds the 10 mm nominal focal length of the objective. While the simplest model of the objective would be a single paraxial lens with a focal length  $f = 10$  mm, such a model would be incompatible with placing optical elements such as windows and iris apertures close to the entry face of the physical objective. To preserve the possibility of modeling such elements, we modeled the objective with two paraxial lenses.

The two-lens objective model is illustrated in Fig. S2. For simplicity, we placed two circular paraxial lenses at the physical ends of the objective body. The diameters of the lenses are equal to the diameters of the entry and exit pupils of the objective,  $\emptyset_1$  and  $\emptyset_2$ , which are given by:

$$\emptyset_1 = 2 WD \tan(\sin^{-1}(NA)) \quad (\text{Eqn. 1})$$

$$\emptyset_2 = 2 \frac{f_{TL}}{M} \tan(\sin^{-1}(NA)) \quad (\text{Eqn. 2})$$

where  $WD$  is the working distance of the objective,  $NA$  is the numerical aperture,  $M$  is the magnification, and  $f_{TL}$  is the focal length of the tube lens.

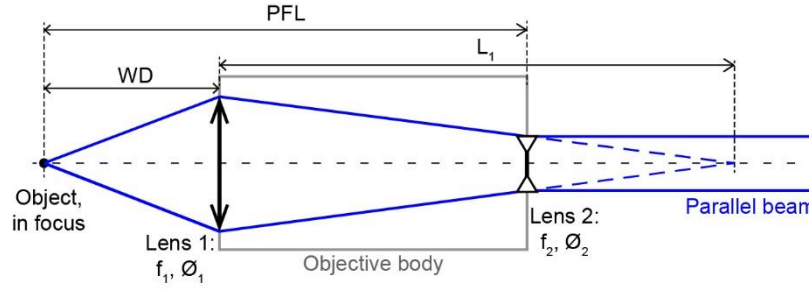

**Figure S2.** Model of the long working distance microscope objective. The objective is modeled with two paraxial lenses at the end of the objective. The lens parameters are determined based on the numerical aperture ( $NA$ ) of the objective and on the formation of a parallel beam from a point source in focus.

The focal lengths of the two lenses,  $f_1$  and  $f_2$ , were calculated based on the requirement that a point light source in the focal plane produces a parallel beam after the second lens. The first lens generates an intermediate image at a distance  $L_1$  after the first lens, which we calculated based on the requirement that the cone of light from the first lens overlaps exactly with the aperture of the second lens. The distance  $L_1$  is given by

$$L_1 = M \times WD \times \frac{PFL - WD}{M \times WD - f_{TL}} \quad (\text{Eqn. 3})$$

where  $PFL$  is the parfocal length of the objective. The focal lengths were then calculated using the lens formula for the first lens, and the condition that the beam is parallel after the second lens. This leads to the following formulas:

$$f_1 = (WD^{-1} + L_1^{-1})^{-1} \quad (\text{Eqn. 4})$$

$$f_2 = -\frac{f_{TL} \times L_1}{M \times WD} \quad (\text{Eqn. 5})$$

For the 20× objective used in this study, we used the nominal values of  $PFL$ ,  $WD$  and  $f_{TL}$  (95 mm, 20 mm, and 200 mm, respectively), and an experimentally measured value of the magnification,  $M = 20.115$ . A

slight difference from the nominal 20 $\times$  is to be expected since our experiments use light with a shorter wavelength than the design wavelength of the objective. With these parameters,  $f_1 = 17.635$  mm,  $\emptyset_1 = 18.512$  mm,  $f_2 = -74.147$  mm, and  $\emptyset_2 = 9.203$  mm.

The two-lens design described here leads to a match between simulated and experimental images that is as good as a single-lens design (see Section 2). It is a conceptually simple solution for modelling a specific objective, but it is not a unique design solution because the two paraxial lenses could be placed elsewhere inside the body of the objective. Different lens placements might lead to a better match with the experiment.

A limitation of our design is that it does not consider the lateral field of view. For high magnification objectives the lateral field of view is much smaller than the lens diameters, and the calculated lens diameters (Eqns. 1 and 2) are close to the physical size of the entry and exit pupils. Therefore, although the formulas given here can be applied to any objective, our approach should be used as a guide rather than a recipe. Depending on the design and construction of a complex optical element, a different strategy might be needed to generate an ideal lens model for it.

### *1.3. The angular corrector*

The angle of incidence of rays on lenses depends on the details of the optical system. In our setup the object is small and located on the optical axis, and the distribution of rays is axisymmetric. For a point source on the optical axis, the angle of incidence on a flat lens surface increases radially as the rays intercept the lens further away from the optical axis. More generally, the angle of incidence will have a radial dependence given by the collimation of the rays and by the lens curvature. For an uncoated lens, the reflection losses are given by Fresnel coefficients, which depend on the incidence angle. An angular dependence is also likely for optics with antireflection coatings. Therefore, light losses through the imaging system are likely to depend on the angle the rays make with the optical axis near the object. Calculation of these angular reflection losses is in general not possible for a corrected microscope objective because it requires a complete knowledge of the objective's construction including the angular efficiency of all optical coatings. Instead, we calibrated these losses experimentally, for the case of objects imaged near the optical axis.

We used an annular aperture with an inner diameter of 2.42 mm and an outer diameter of 3.18 mm to divide the light cone into 9 ranges of angles with respect to the optical axis, from 0° to 26.7°. This was done by setting the pinhole for light field calibration at the location of the drops, followed by placing the aperture at different distances behind the pinhole, calculated such that the angular intervals over which the light could pass added up to the full angular range without overlapping. Rays with angles between 0° and 4.2° could not be measured with the annular aperture, and the data point for this angular range was extrapolated from the other measurements. The data point for the interval between 21.1° and 26.7° was also extrapolated because the experimental illumination dropped to negligible levels within this interval. The relative angular efficiency of the imaging system in each angular range was obtained by dividing the total light intensity observed through the imaging system by the light intensity right after the aperture, then normalizing these values such that the largest value was equal to 1. The intensity after the aperture was measured with a camera placed directly after the aperture and corrected for the camera's angular efficiency.

In the model, the angular correction was implemented using an angular corrector built from concentric adjacent rings. The inner and outer diameters of the rings were calculated to correspond to the angular ranges of the experimental calibration, and each ring had a light transmission ratio equal to the relative

angular efficiency measured experimentally. All the rings were placed in the same plane, at a position that corresponds to the closest calibration distance between the image plane and the annular ring.

#### 1.4. Other components

The remaining elements in the model were the tube lens and the camera. The tube lens was modeled as a paraxial lens with a focal length of 200 mm, the same as the nominal focal length of the physical lens. The actual focal length of the tube lens depends on the wavelength, but we used the nominal focal length because using it replicated the measured optical magnification. Small deviations from the nominal focal length values were accounted for by using an experimental magnification value in the design of the objective, rather than the nominal magnification (see Section 1.2.).

The camera was modelled with a virtual camera with pixels of the same size as the pixels in the physical camera,  $10\text{ }\mu\text{m} \times 10\text{ }\mu\text{m}$ . The pixels of the virtual camera count all the rays that intercept them (*i.e.*, a “ray hit”). The pixel number and aspect ratio of the virtual camera were chosen to generate a simulated image with region of interest close to the one used in experiments.

## 2. Ray-tracing model testing and characterization

To test the accuracy of the model, we compared experimental focus scans of spherical water drops with several variations of the ray tracing model. These comparisons are shown in Fig. S3 and include different focus positions than the ones shown in the main text, Fig. 2. For the additional positions, the agreement with the experiment remains very good, but slight differences are evident at  $-40\text{ }\mu\text{m}$ .

Figure S3 also shows simulated images from a model that replaces the two-lens objective with an  $f = 10\text{ mm}$  paraxial lens. The two models for the objective produce simulations that are indistinguishable from each other, so the two-lens design is not essential for the accuracy of the model. Nevertheless, we chose to use the two-lens design because it replicates the working distance of the physical objective.

In the next model variation we tested, we removed the angular corrector. In this case, the simulated images became slightly different, and their match with the experimental images was degraded. This degradation is difficult to see in images, but it becomes apparent if the image is projected onto a line. Therefore, the angular corrector is necessary to improve the accuracy of simulations.

The next series of images in Fig. S3 were obtained with mismatched light field sources: illumination with slightly different LED settings (50 ns pulses instead of 100 ns), and with an imprecise light field for the laser illumination (see Section 5.3.). Despite the illumination background being highly uniform in the image, the match with the experimental images is degraded. The dependence on the light field duration of the LED pulse was surprising, and highlights the necessity of using a light field illumination source that is calibrated experimentally.

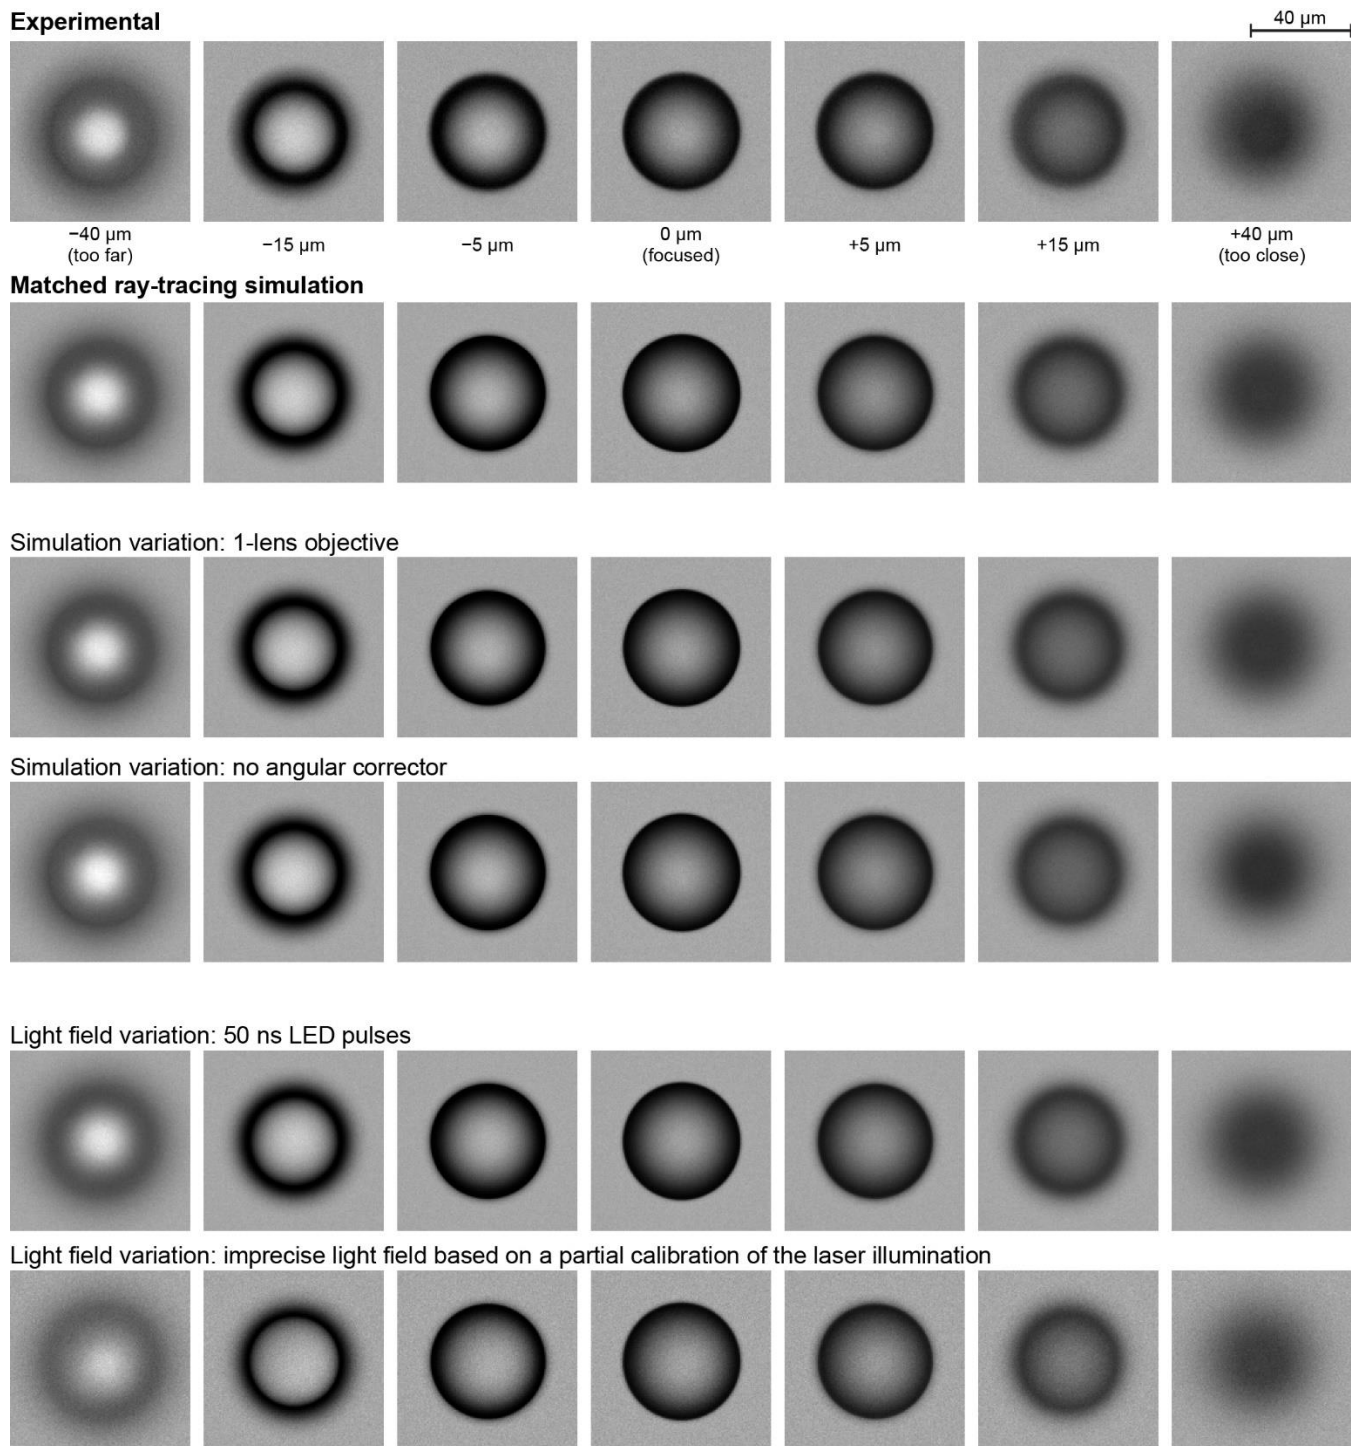

**Figure S3.** Extended focus scans of spherical water drops, for several variations of the model and of the light field source. The top row shows the experimental images, the next rows simulated images, and the listed distances give the relative position of the drop in the direction of light propagation. Small differences between images are best seen on a computer screen.

### 3. Computation times

Simulating images with the same number of ray hits as the number of photons captured in the experimental images is an intensive computational task. For example, the droplet merging images were simulated with a virtual sensor size of 200 by 300 pixels, and the experimental images have a signal that corresponds to around 2500 photons per pixel. To replicate the experimental image with the same ray number,  $200 \times 300 \times 2500 = 150$  million ray hits are needed. Since only part of the rays from the source arrive at the detector, around 400 million rays had to be traced from the source. On our 64-core workstation (Lenovo P620 with an AMD Ryzen ThreadRipper PRO 3995WX processor), simulating one image took approximately one hour.

Computation times increase significantly when tracing rays through drops with pressure waves, primarily due to the refractive index distribution, which is not uniform. To consider the variations in refractive index with high accuracy, the ray path must be calculated in much smaller length steps than for a homogenous object, and this increases the computational time. Additionally, the size of refractive index data impacts the speed. The refractive index data is stored in a .dll file with the format needed in Zemax, as discussed in Section 5.3. For axisymmetric drops, the refractive index distribution can be efficiently represented in a 2D matrix because the 3D distribution can be calculated using the symmetry of the drop, resulting in relatively small files and only a small increase in the computation time. If the drop is not axisymmetric (see Section 6.3.), a 3D matrix is required to store the refractive index distribution. This leads to larger file sizes and substantially longer computation times. Furthermore, if the drop does not have a basic shape available in Zemax, a virtual surface stored in an .stl file must be used (see Section 4.3.). This can significantly increase the computation time, especially if the surface is highly resolved. The most complex simulations, with 3D refractive index and surface data, were used for the main text Fig. 4 and Supplementary Movie 5 and required around 10 hours of computations per image.

Although the computations are lengthy, ray tracing is parallelizable with a linear speed gain, which allows efficient use of multi-core workstations, computer clusters, or cloud computing. Also, in some applications it may be sufficient to simulate images with much fewer ray hits than photons. Here, to explore how well ray tracing replicates experimental images, we used simulations with the same number of rays as photons. However, the sensitivity of measuring a feature in the image can be increased by integrating the light intensity over the feature, which can decrease substantially the noise. If a 10 times higher image noise is acceptable in simulations, the number of rays that must be traced decreases 100-fold, because the relative shot noise scales with the inverse square root of the number of rays.

## 4. Focus scans and triple droplet merging

### 4.1 Experimental details

The droplets used in the focus scans and in the triple drop merging were generated in air using a 20  $\mu\text{m}$  diameter nozzle (MicroFab MJ-AT series) equipped with a piezoelectric element that triggered the Rayleigh breakup of the jet produced by the nozzle. The nozzle was fed from a water reservoir pressurized with compressed air, and the nozzle back pressure was 0.1 MPa. The nozzle was oriented such that the drops moved vertically downwards and passed through the imaged region after several millimeters of flight, during which the drop oscillations occurring after the jet breakup damped. The nozzle was surrounded by a sheath of dry air, and the drops evaporated during flight, which made them cool slightly below the room temperature. Using an evaporative cooling model [23, 24] we estimated that the merging drops had a surface temperature of 16 °C (289 K) when they merged.

For the focus scans, the droplets were synchronized with the LED source and the camera by exciting the nozzle in phase with the LED and the camera, which made different drops appear in the same position in the camera images. The nozzle was operated with a sinusoidal wave with an amplitude between 1.2 and 4 V<sub>pp</sub>, and a frequency of 72 kHz, which is a multiple of the 500 Hz frequency of the LED and camera triggers. This setup produced drops with constant diameter and velocity, which travelled equally spaced and arrived at the imaged region with a uniform rate.

For the drop merging experiments, the piezo signal was modified to generate periodically groups of drops with slightly different velocities, which made them collide and merge during flight. The change of velocities is based on the relationship between drop velocity and the amplitude of the piezo voltage. For our nozzle, the velocity of drops increased as the amplitude of the driving signal increased. Therefore, the drop velocities can be modulated by applying an amplitude modulation (AM) on the piezo signal.

To generate groups of N drops, the frequency of the modulation should be equal to the droplet frequency divided by N. To generate groups of three drops, we applied on the sinusoidal 72 kHz driving signal an amplitude modulation at  $72 \text{ kHz}/3 = 24 \text{ kHz}$ . If the droplets would respond instantaneously to the change in the voltage amplitude, an increasing triangular ramp AM modulation would be sufficient. In practice, the response of our nozzle was gradual, and we found that a decreasing rather than an increasing ramp was needed to generate merging drops. However, the ramp AM produced relatively small velocity differences, and the drops needed to travel long distances before merging, which made the merging less reproducible. To obtain the largest modulation of the drop velocities, we used a square modulation with AM levels at 100% and 0%. With the square AM modulation, it was also possible to adjust the relative velocity of the drops by changing slightly the phase of the modulation. Figure S4 shows the waveforms used to generate groups of two and three merging drops. We found empirically that a waveform that works well has an AM duty cycle of 50%, with the zero phase of the AM being simultaneous to the zero crossing of the sinusoidal nozzle signal.

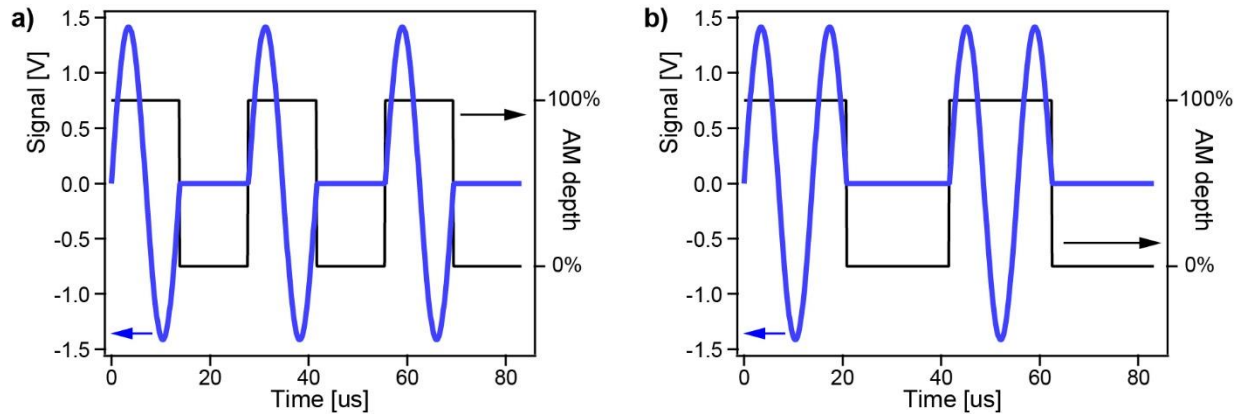

**Figure S4.** Nozzle voltages applied to generate (a) two merging drops and (b) three merging drops. The frequency of the sinusoidal signal is 72 kHz.

The generation of merging drops was less reproducible than the generation of single drops. The merging time of the drops had a jitter of approximately  $0.75 \mu\text{s}$  peak to peak, one order of magnitude less stable than the arrival time of single drops. Besides introducing a temporal uncertainty, the timing jitter caused some drop triplets to collide sequentially rather than simultaneously, and led to asymmetric shapes during merging. The synchronization of the drop collisions degraded on a timescale of minutes, most likely due to small variations of the nozzle temperature and pressure, and we adjusted the AM phase manually to

maintain simultaneous collisions and symmetric merging. The drops from the colliding group had slightly different travel directions, leading to collisions in which the drop centers were not perfectly in line, and to a rotation of the merged drops. The rate of rotation was relatively slow, and the rotation was barely visible. For experiments with the merging drops in focus, the axis of rotation was along the imaging axis, and it can be discerned in the last frames of Supplementary Movie 1. In the experiments with the merging drop traveling across the focal plane, the rotation axis was perpendicular to the imaging direction and cannot be seen directly. However, Supplementary Movies 2 and 3 are consistent with a rotation of approximately  $1^\circ$  during the duration of the movies (see Section 6.2.).

To image the drop merging process, the frequencies of the LED and camera triggers were changed from 500 Hz to 499.997 Hz. This led to a slow drift of the phase of the images, and the camera displayed live the merging process at a greatly slowed rate. The raw movies of the drop merging were recorded in this mode. For analysis, we selected from these movies a series of images that (i) showed symmetrically-merging drops generated by simultaneous collisions, and (ii) covered most of the distinctive drop shapes observed up to approximately 30  $\mu\text{s}$  after the initial contact. The later criteria led to a nonlinear increase of the frame's time delay with the number of the frame.

#### *4.2. CFD simulations for droplet merging*

We performed numerical simulations of the merging droplets using the compressible multiphase flow solver ALPACA [15] and the robust discrete-equations method with interface capturing (RDEMIC) [25]. Although this method employs a diffuse-interface approach, the interface can be accurately reconstructed, tracked, and extracted for post-processing. Since the interface dynamics during the merging of the droplets is dominated by surface tension, the curvature is computed from the reconstructed interface as well.

Both fluids, atmospheric air and water, were modelled with the stiffened-gas equation of state (EOS) [20]. The EOS parameters were  $\gamma = 7.15$ ,  $P_\infty = 3.046 \times 10^8$  Pa for water, and  $\gamma = 1.4$ ,  $P_\infty = 0$  Pa for air. To match the experimental conditions at  $P = 101325$  Pa and  $T = 289$  K (see Section 4.1.), the initial densities for water and air were  $999 \text{ kg/m}^3$  and  $1.222 \text{ kg/m}^3$ , respectively. The surface tension was set at  $\sigma = 0.073344 \text{ N/m}$  for water at 289 K [26].

In the experiment, the three droplets moved and collided almost collinearly. Therefore, the simulation was performed in 2D with enforced cylindrical symmetry around the collision axis to reduce computational costs. The setup was further simplified by enforcing symmetry between the outer droplets with respect to the center droplet. Thus, only one outer drop with radius  $r_O = 22.2365 \mu\text{m}$  and half of the central drop with radius  $r_C = 22.5617 \mu\text{m}$  were simulated. The center drop was at rest, and the outer drop moved towards it with  $u = 0.222 \text{ m/s}$ . The drops were initialized such that they exactly touched each other. The adaptive cartesian mesh used about 125 cells per initial drop radius at its finest resolution.

#### *4.3. Generation of virtual non-spherical drops for image simulations*

For the single droplet focus scans the drops were modeled as a sphere (a basic object that is available in Zemax). For the drop merging and for the drop ablation simulations, a 3D virtual object must be generated. The 3D object has a bounding surface where rays refract, and a volume which may have refractive index variations that bend the rays.

Computationally, the virtual 3D objects for the merging drops simulations were composed of (i) a surface object and (ii) a volume object with a constant refractive index. The refractive index was equal to the refractive index of water at ambient conditions and the wavelength of the illumination light.

The surface objects for the droplet merging simulations were created by revolving drop outlines from either experimental images or CFD simulations. The experimental images were saved as .tiff files to prevent file compression losses, and their resolution was enhanced 5×5-fold by using the image scaling function from Adobe Photoshop (version 26.8.1) with the bilinear scaling algorithm, which we found to preserve best the image details. The edges of the drops were then extracted from rows or columns of pixels, as the pixels where the light intensity dropped to 50% of the background level. This procedure generated a set of pixels that marked the edge of the drop, from which we extracted a set of points in the image plane, with coordinates calculated using the image magnification (0.497  $\mu\text{m}/\text{pixel}$ ).

The surfaces of the merging drops were generated in Autodesk Inventor (2025, February release) using the digitized outline of the experimental drop (*i.e.*, the set of edge points). The spline and line connection tools from Autodesk Inventor were used to generate a line object that traced the drop edge. Since the three drops were not in a line when they collided, the line object was not symmetric relative to the axis defined by the drop contact points, and a 3D surface could not be generated by a simple revolution. Instead, we divided the line object in two halves and revolved them separately by  $\pm 90^\circ$  relative to the image plane. This procedure has the advantage that it approximates well the curvature of the object near the image plane, while preserving most of the asymmetry of the real object. The disadvantage is that the two revolved halves do not join smoothly. Since the joining plane is along the viewing direction, the impact of the mismatch in the simulations is minimized, but significant differences from the experimental images can emerge for some drop shapes.

We modified the regions near the joining plane by “shaving” the object near the jumps to remove the discontinuities in the surface, and exported the smoothed object as a .stl file. The .stl file was then imported into Autodesk Fusion (version 2602.1.25), where the object mesh was smoothed and regenerated at a higher resolution. The regeneration corrected errors in the stitching of the two halves, which could make a line appear in the image simulations. Mesh smoothing and regeneration produced a high-resolution 3D surface that replicated the cross section of the object in the image plane. This surface was exported as a .stl file and imported in Zemax for ray tracing.

For the CFD-simulated merging drops, the CFD results included the outline of the drop as a line saved in .stl format. Since the CFD simulation is axisymmetric, the outline traced only one half of the drop. The drop outline was completed based on the symmetry of the simulation, and the 3D surface object was generated by revolving the outline in Autodesk Inventor.

Since the experimental images have an estimated time delay error of  $\pm 0.75 \mu\text{s}$ , longer than the time in which significant drop shape changes can occur, the time points for ray-tracing simulations of CFD drops were selected based on the shape of the drops rather than on the time delays. The CFD drop shapes were extracted every 100 ns, and from this data we extracted the most closely matching image for each experimental frame shown in the movies.

## 5. The X-ray laser ablation of water drops

### 5.1. Experimental details

The droplet ablation experiments had the same general setup as in our previous spallation study [16], and was conducted in the Coherent X-ray Imaging (CXI) endstation [13] at the Linac Coherent Light Source [17]. The water droplets were generated from a 20  $\mu\text{m}$  diameter nozzle equipped with a piezoelectric element (MicroFab MJ-AT series), operated at a back pressure of 0.097 MPa. The nozzle piezo was driven with a square wave with 49% duty cycle, 4.1 Vpp amplitude, and a frequency of 71.42857 kHz. This frequency is twice the frequency of one of the X-ray laser's timing clocks and synchronizes the drops to the X-ray pulses. Due to the finite resolution of the frequency setting of the function generator, the frequency of the nozzle could not be matched exactly to the X-ray pulses. As a result, the phase difference between the drops and the X-ray pulses drifted slowly, and the phase of the nozzle signal was adjusted manually to keep the droplets aligned with the X-ray pulses.

The droplets were injected into a vacuum chamber, pumped down to a fraction of 1 Torr via the roughing vacuum line at CXI. The turbopumps were turned off to minimize mechanical vibrations that reduce the probability that a droplet is intercepted by the X-ray laser pulse. The droplets cooled by tens of degrees Celsius before being intercepted, and we used an evaporative cooling model [23, 24] to calculate the temperature distribution of the droplets at the moment of ablation.

The X-ray pulses were focused using compound refractive lenses (CRLs) to change the focused beam size. The CRL's refractive index and focal length vary with the X-ray energy, therefore tuning the X-ray wavelength moves the focus along the beam and changes the size of the beam at a fixed position. Using X rays near 12.4 keV, the diameter of the beam at the drop could be varied from approximately 2 to 4 microns. With a larger diameter beam, the energy deposited by X rays is distributed over a larger volume and the temperature of the heated filament decreases, which allowed us to reach the regime where visible pressure waves were generated but the region exposed to X rays remained liquid.

The average energy of the X-ray pulses at the point of generation was approximately 0.5 mJ, but the pulse energy at the sample was lower than this due to losses along the beamline and in the X-ray optics. Based on the properties of the beamline, and on comparisons to a drop ablation experiment with known pulse energies [19], we estimated a transmission factor between 0.1 and 0.25.

The two ablation experiments discussed here had different settings. For the ablation experiment that did not produce an ablation hole, the droplets traveled 10 mm from the nozzle with a velocity of 10.4 m/s, at 620 mTorr pressure, and had an average temperature of  $-10^\circ\text{C}$  when intercepted by the X rays. The X-ray photon energy was 12.3 keV and the X-ray beam had a diameter of 3.8  $\mu\text{m}$  FWHM (measured by imaging the X-ray fluorescence in a YAG:Ce scintillator crystal).

For the ablation experiment that produced an ablation hole, the droplets traveled 4 mm from the nozzle with a velocity of 10.2 m/s, at 350 mTorr pressure, and had an average temperature of  $1.2^\circ\text{C}$  when intercepted by the X rays. The X-ray photon energy was 12.4 keV and the X-ray beam had a diameter of 1.9  $\mu\text{m}$  FWHM.

### 5.2. CFD simulations of drop ablation

The computational fluid dynamics (CFD) simulations utilized the Noble-Abel Stiffened-Gas (NASG) equation of state (EOS), with coefficients computed to match the thermodynamic properties of water [20]. To improve the accuracy of our CFD simulations, we further optimized the coefficients of the

NASG EOS to match the thermodynamic properties predicted by the empirical EOS of water given by International Association for the Properties of Water and Steam (IAPWS-95) [21].

The optimization was performed for the conditions of our ablation experiments, where liquid water undergoes shock compression and adiabatic compression starting from specific temperatures and pressures. Since the experimental data is highly sensitive to the speed of the pressure waves, the criteria for optimization were (i) having the same density at the initial temperature and pressure as predicted by IAPWS-95, and (ii) the minimization of differences between the speeds of sound and shock waves predicted by NASG and IAPWS-95.

The pressure-density-temperature relation in the NASG EOS has four coefficients. We optimized three of these coefficients: (a) the specific heat of water at constant volume  $C_v$ , (b) the adiabatic index  $\gamma$ , and (c) the co-volume  $b_{vol}$ . The fourth parameter is the stiffened pressure  $P_\infty$ , which becomes a dependent variable that is calculated from the other three parameters, because the initial density is constrained to the IAPWS-95 value. The objective function minimized during optimization was the sum of the mean squared relative differences in  $c_0$  and  $c_s$ :

$$\text{Err}(\rho_{OPT}; C_v, \gamma, b_{vol}) = \text{mean} \left( \left( \frac{\Delta c_0}{c_{0,IAPWS}^{IAPWS}} \right)^2 \right) + \text{mean} \left( \left( \frac{\Delta c_s}{c_{s,IAPWS}^{IAPWS}} \right)^2 \right) \quad (\text{Eqn. 6})$$

where  $\rho_{OPT}$  is a list of densities (900–1355 kg/m<sup>3</sup>, in steps of 1 kg/m<sup>3</sup>) and  $\Delta c_{0,S} = c_{0,S}^{IAPWS} - c_{0,S}^{NASG}$  are the differences in speed and shock velocities at a given density point.

The error function was minimized using MATLAB’s “fmincon” optimization algorithm. This was done separately for each ablation experiment, because the initial water temperature was different. For optimization, we used as the reference temperature the average temperature of the drop calculated from the evaporative cooling model (see Section 5.1.). The reference pressure was the vacuum chamber pressure, which was measured experimentally. After optimization, the adiabatic compression curves approximated substantially better the IAPWS-95 compression data than the ones calculated from the original [20] NASG EOS. The adiabatic compression curves are shown in Fig. S5.

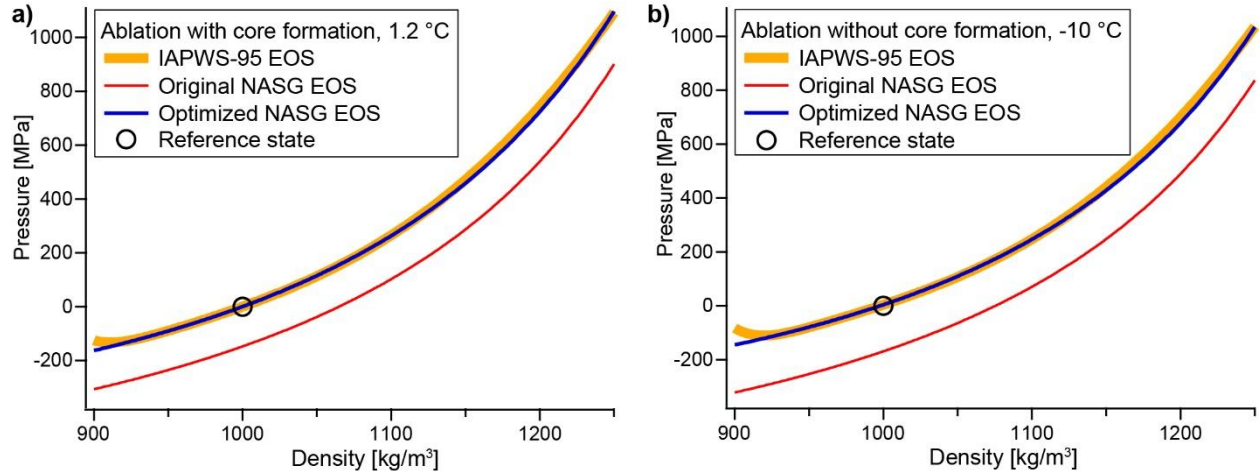

**Figure S5.** Equations of state used in the CFD simulations. The NASG equation of state was optimized to match the IAPWS-95 data at the average temperature of the drops. The graphs display the adiabatic compression curves, starting from a reference point at the experimental pressure and temperature, for the two ablation experiments investigated.

We performed computational fluid dynamics (CFD) simulations using the compressible multiphase flow solver ALPACA [15], to model numerically the ablation of a water drop subjected to intense X-ray pulses. Previous work showed promising results with a similar setup [18]. These simulations model the propagation and reflection of pressure and shock waves inside the drop, starting from an initial condition where a large-pressure cylindrical core is initialized numerically inside a drop at ambient conditions. The simulations provide the pressure and density distributions during ablation, and the position of the surface of the drop (which defines the shape of the drop during ablation). Simulations with different initial conditions were conducted for the experiments with formation of an ablation core, and without formation of an ablation core. If the core formed in the experiment, the simulation used a cylindrical gaseous core, and if it did not, it used a cylindrical liquid core. The symmetry axis of the liquid core passed through the center of the drop, rendering the setup cylindrically symmetric, and the CFD simulation was computed in 2D. In other simulations, the gaseous core was displaced by 2  $\mu\text{m}$  from the center of the drop to match experimental data (see Section 6.3.). In that case, the CFD simulation had to be computed in 3D.

The pressure profile within the core,  $P_{\text{core}}$ , was defined using a Gaussian distribution,

$$P_{\text{core}}(r) = P_{\text{peak}} * \exp\left(-\frac{2r^2}{r_{\text{core}}^2}\right) \quad (\text{Eqn. 7})$$

where  $r$  is the radial position coordinate of the cylindrical core,  $r_{\text{core}}$  is the radius of the core, and  $P_{\text{peak}}$  is the peak pressure inside the core. We determined the parameters of the core,  $r_{\text{core}}$  and  $P_{\text{peak}}$ , according to the criterion that the experimentally observed change in the drop size during the shock reflection [16] was replicated as close as possible by the numerical simulations. Figure S6 shows the comparison between the simulated and experimental changes in radii. We favored replicating the slope of the data over the amplitude, because the slope gives the shock pressure, while the amplitude is a measure of the shock duration. The best matched simulations have slightly earlier dynamics than the experiments, which could be due to the experimental time zero being up to 1 ns too late.

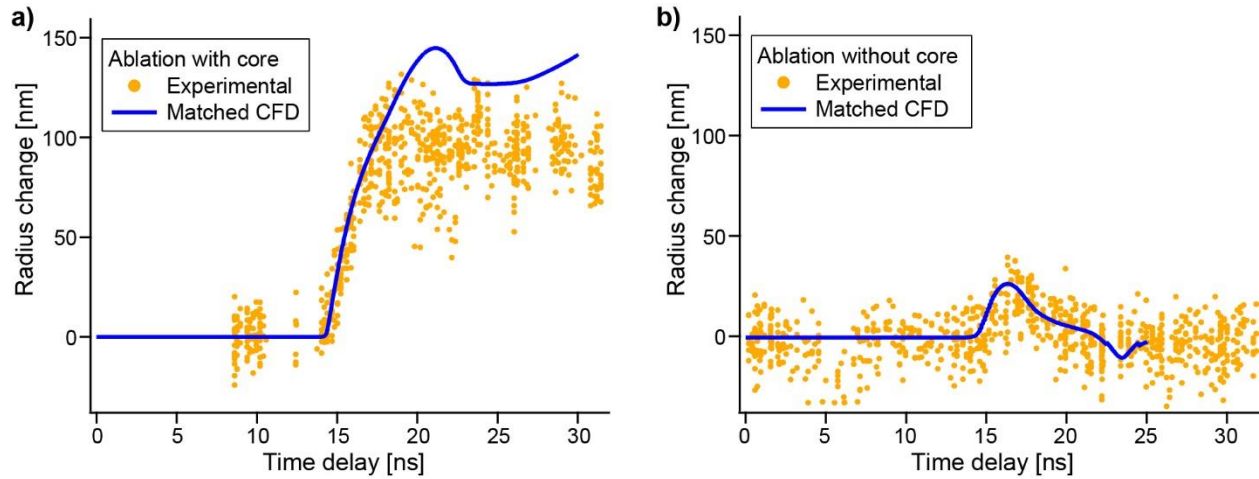

**Figure S6.** Experimental and simulated motion of the drop surface during the reflection of the shock.

The initial pressure and density distributions across the rest of the drop were defined according to the experimental temperature gradient, by setting the pressure equal to the vacuum chamber pressure and by calculating the density distribution from this pressure and the temperature distribution, using the optimized NASG EOS. The surrounding environment was modeled as a gas of water vapor at the pressure of the vacuum chamber.

Examples of the pressure distributions from the CFD simulations are shown in Figure S7 for both ablation experiments. To illustrate the differences in wave amplitudes and signs, the pressure range is the same in both plots, and time delays are the same as for the data shown in Fig. 4 in the main text. The outgoing pressure wave (5 ns) in the experiment that generated an ablation hole started to sharpen into a shock, while in the other experiment the outgoing pressure wave remained smooth. In both cases, the reflected pressure waves (23 ns) reached large negative pressures. The experiment that did not generate an ablation hole had weaker pressure waves, which is consistent with the fact that they were less visible.

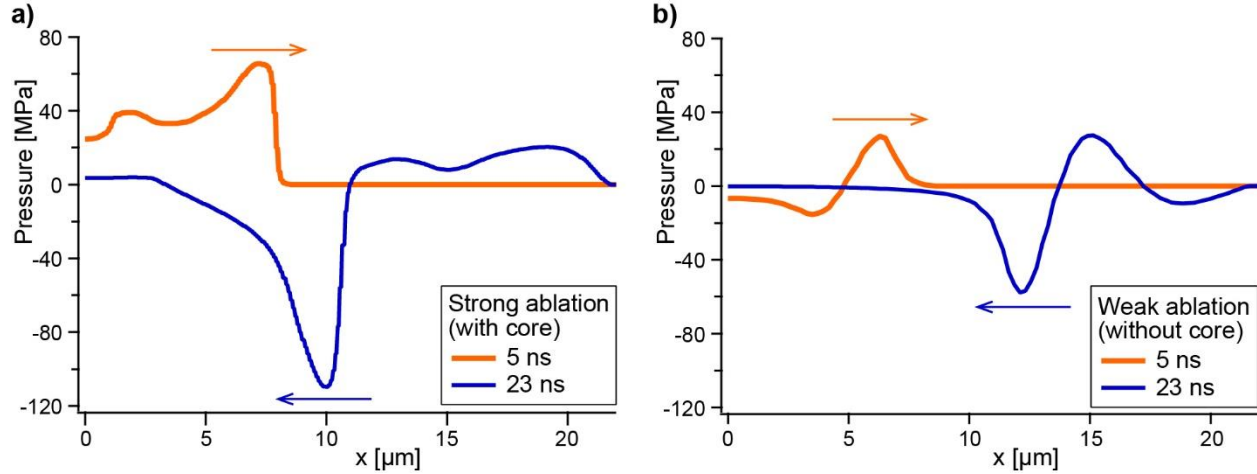

**Figure S7.** Profiles of pressure waves during ablation experiments, along a horizontal line passing through the center of the heated core. a) Pressure profiles for the experiment that generated an ablation hole. b) Pressure profiles for the experiment that did not generate an ablation hole.

### 5.3 Image simulations of drop ablation

The vacuum chamber used in the ablation experiments did not have the space needed to insert the camera and measure the light field (see Section 1.1.). Therefore, after completing the experimental data collection, the optical setup was replicated on an open optical table to characterize the light field. The calibration was different, in terms of the recorded surfaces, from the one described in Section 1.1. The first surface was the image of the light beam after the condenser lens, with the camera chip positioned as close as possible to the condenser. The second surface was the image of the entire illumination beam at the image plane. Ray tracing between these two surfaces yielded a less accurate model of the light field. Since the surfaces recorded the full cross section of the illumination beam, there were spatial and angular correlations between the light intensity on the two surfaces, which were not replicated when the rays were traced randomly between surfaces. The light field determined by this method replicated poorly the images of the focus scan, so it could not be trusted to produce high-fidelity image simulations.

To approximate better the experimental illumination, we used a light field produced by the LED light source through the same illumination setup. We surveyed different settings on the LED, which produced different light fields, and we found that when the LED pulse width was 50 ns, the corresponding light field produced simulated images of the drops that closely matched those captured experimentally with the femtosecond laser.

The surfaces of the drops from axisymmetric ablation simulations were generated by revolving the CFD-simulated drop outline in Autodesk Inventor, following the same procedure used to generate the surface of CFD-simulated merging drops (see Section 4.3.). The drop outline was extracted from a plot of the drop

density in a plane that passes through the drop's center, as the region where the drop density becomes lower than  $900 \text{ kg/m}^3$ .

The surfaces of the drops from non-axisymmetric ablation simulations were created by extracting one quarter of the drop surface from the CFD simulation, and exporting it to a .stl file. The resolution of the CFD surface was higher than needed and this slowed down significantly the image simulations, so we scaled down the triangulation density to 5% of the original density. The scaling down was done with the "adaptive remesh" option such that small features of the cavitation hole did not disappear or lose smoothness. We tested different scaling factors, and we chose the maximum reduction that preserved the appearance of the simulated images.

The refractive index distribution inside the liquid drop was calculated using the IAPWS R9-97 formula [22], which gives the refractive index of water based on the water density and temperature, and the wavelength of the light. The density and pressure distributions in the liquid were obtained from the CFD simulations, and from them the temperature distribution was determined using the optimized NASG EOS (see Section 5.2.). The refractive index distribution was then padded, in the gaseous regions, with the refractive index at the initial pressure and temperature. The padding ensured that there were no gaps with low refractive index between the boundary of the volume describing the liquid and the surface object described in the previous paragraph. Finally, the refractive index data was used to create a dynamic-link library (.dll file) that described, in the format used by Zemax, the object and its refractive index distribution. The refractive index file and the surface files were then imported in Zemax to define the virtual drop in the ray-tracing model.

The ablation core was not empty, as the time delays investigated were too short for the vapor to escape, and images simulated assuming the core was empty had a higher contrast of the core feature than in the experiment, especially at shot time delays. We therefore estimated a constant density of the water in the core (and from this, the corresponding refractive index) by assuming that the core material was conserved and its density decreased according to the experimental increase of the diameter of the core. The 3D surface of the drop was separated into an outer-drop surface and an inner-core surface to generate a liquid drop object and a core object in Zemax, with the core object imposed on top of the liquid drop object, which had the refractive index distribution described in the previous paragraph.

## **6. Sensitivity, accuracy, and impact on fluid dynamics simulations**

### *6.1. Potential for constraining wave pressures*

To evaluate if combined CFD and image simulations can be used to constrain the wave pressures, we simulated additional images of the shock wave shown in the main text Fig. 4, for CFD simulations with lower and higher filament pressures. The simulated images for default, lower and higher pressures are shown in Fig. S8(a) along with the experimental image. The agreement with the experimental image became worse for the higher and lower filament pressures, which led to shocks with amplitudes around 10 MPa below and above the best-matched simulation. Thus, for this example, image simulations can help constrain the shock pressure within  $\pm 10 \text{ MPa}$  based on visual comparisons. The accuracy with which the pressure can be constrained visually in Fig. S8(a) was limited by (i) the experimental noise, which was larger for the present data than in previous studies [19], and by (ii) the imperfect calibration of the illumination's light field.

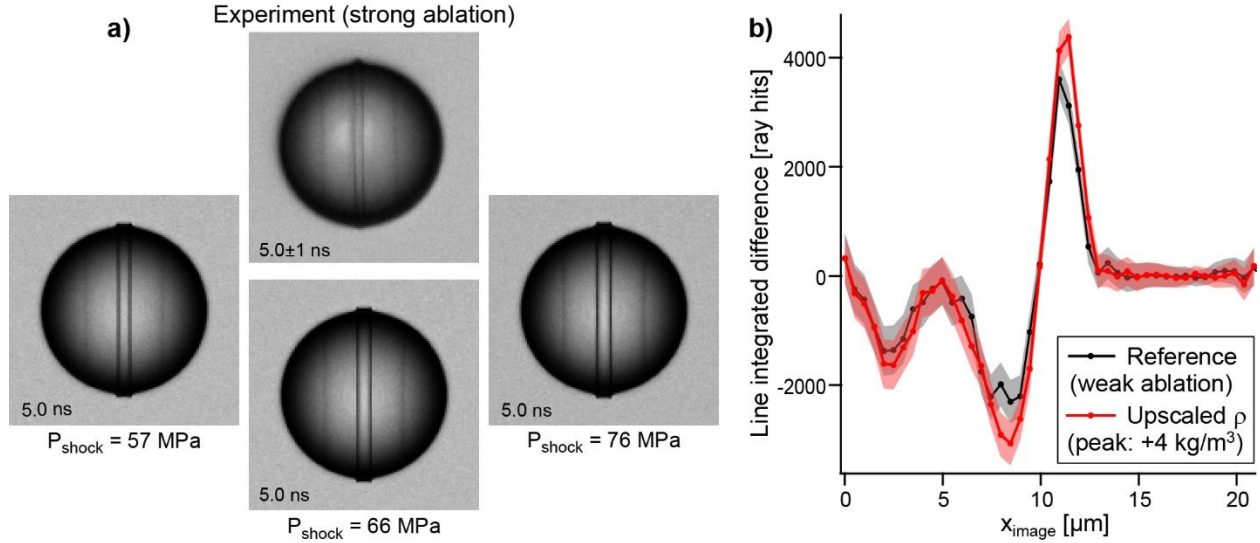

**Figure S8.** Constraining pressure wave amplitudes with image simulations. (a) Experimental image of a shock wave from the strong ablation experiment, and images simulated for different initial conditions in the CFD. Shocks with peak amplitudes around 10 MPa different from the best matching conditions lead to a degradation of the match between simulation and experiment. (b) Integrated difference profiles of image simulations for the weak ablation experiment, for the best matching simulation and for another simulation with a linearly upscaled density distribution. For a density distribution with a peak increase of 4 kg/m<sup>3</sup>, the peaks of the profiles differ more than expected shot noise, which is indicated with color bands at  $\pm 1$  standard deviation.

We also evaluated the sensitivity of discriminating different pressure amplitudes in simulations. As a reference, we used the 5 ns CFD simulation for the weak ablation case, which produces image features that are barely visible (see Supplementary Movie 4). We then scaled linearly the difference between the wave density and the initial density such that the peak density in the wave increased by a fixed amount, and conducted image simulations for drops with the upscaled density distribution. To decrease the shot noise and increase sensitivity, we integrated a horizontal slice in the image and subtracted it from the integrated intensity profile for a drop in the initial condition.

Figure S8(b) shows the line integrated image differences for the reference shock wave image, and the density-upscaled image. The band around the profiles represents the standard deviation of the data due to shot noise, calculated as the square root of the sum of ray hits in the shock image and the reference image. The profile for a shock with peak density upscaled by 4 kg/m<sup>3</sup>, corresponding to a pressure variation of 8 MPa, is significantly different than the profile for the reference shock. This sensitivity can be improved by reducing the shot noise via using more rays in the simulation, which in the experiment corresponds to using higher illumination intensities. For the experimental setup we used, the illumination intensity can be improved by at least one order of magnitude by using higher energy laser pulses, a tighter illumination spot, and a higher pixel magnification to prevent the saturation of the camera. With an order of magnitude higher illumination intensity, peak density changes around 1 kg/m<sup>3</sup> should be detectable.

### 6.2. Observation of small rotations of the merging along the imaging direction

The system of the three merging drops rotated during flight. The rotation angles were slight, and the orientation of the rotation axis varied between experiments. In the in-focus movie of the merging drops (Supplementary Movie 1), the axis of rotation was along the imaging axis and the drops rotated counterclockwise in the image. The accumulated rotation during the movie was small, so it is best seen in the last frame, by comparing the experimental drop to the CFD simulated one (which did not rotate).

The merging drops that were imaged while traversing the image focal plane also rotated, but the rotation was perpendicular to the imaging direction, thus the rotation was not directly visible. When we generated simulated images of these drops, we varied the tilt angle made by the imaging plane with the direction of travel of drops. We found that the best match with the experiment was achieved for tilt angles of  $4^\circ$  and  $5^\circ$ , and that the first frames are better matched at  $5^\circ$  while the last frames are better matched at  $4^\circ$ . This observation suggests that the drops rotated by approximately  $1^\circ$  during the observation period.

The rotation observed using image simulations was consistent with the injector setup and the kinematics of the droplets before merging. The droplets made contact after around  $500\ \mu\text{s}$  and  $5\ \text{mm}$  of flight, since the approximately  $40\text{-}\mu\text{m}$  diameter drops started separated by approximately  $140\ \mu\text{m}$  center-to-center, and the top and bottom droplets were about  $0.2\ \text{m/s}$  faster and slower than the center droplet, respectively. Using the imaging and injector angles, we deduced the approximate centers of the droplets before collision with respect to one another to calculate the initial total angular momentum. The angle of the injector to the imaging plane, and thus the initial angle of droplets during flight, was set at  $8^\circ$ . Since just before merging the drops were best replicated by a simulation at an angle of  $5^\circ$ , this implies that the droplets rotated  $3^\circ$  before touching, in the same direction as the rotation deduced from image simulations. Taking this  $3^\circ$  rotation, the centers of the droplets were about  $2.3\ \mu\text{m}$  above and below the injector plane at the time of contact, and their velocity relative to this plane (which is approximately the tangential velocity in the rotation frame) was  $(2.3\ \mu\text{m})/(500\ \mu\text{s}) = 4.6\ \text{mm/s}$ . We then considered the three droplets as spheres with the measured  $44.42$ ,  $45.12$ , and  $44.52\ \mu\text{m}$  diameters (from top to bottom) to calculate the initial moment of inertia and the initial angular momentum. After collision, we tracked the rotation by using these initial conditions and moment of inertia matrices extracted from our stl models of the merging drops in Autodesk Fusion. Using 20 discrete moments of inertia calculated during the roughly  $30\ \mu\text{s}$  process, we calculated the corresponding angular velocities using the conservation of angular momentum. We then integrated numerically the discrete angular velocities, which resulted in a rotation angle of  $0.73^\circ$  during the first approximately  $30\ \mu\text{s}$  of the merging process.

### 6.3. Determining slight misalignments between the drop and the X-ray pulse

In the drop ablation experiments the X-ray pulse should pass through the center of the drop, but micron-scale misalignments can occur. Such misalignments are difficult to detect if they occur along the imaging direction, but the image of the negative pressure wave is sensitive to them. For the ablation movie that generated an ablation hole, we initially used an axisymmetric CFD model, and the corresponding simulated images did not reproduce the aspect ratio of the negative pressure wave.

To determine the experimental misalignment, we performed non-axisymmetric CFD simulations where the core axis was displaced from the center of the drop along the imaging direction. Figure S9 shows the experimental image from main text Fig. 4, along with corresponding simulated images for misalignments ranging from  $0\ \mu\text{m}$  to  $4\ \mu\text{m}$  (in the direction of light propagation). The best match was obtained with the core misaligned by  $2\pm 1\ \mu\text{m}$ . Same as in the case of the rotating drops (Section 6.2.), high fidelity image

simulations allowed the quantification of minute details that are difficult to detect because they occur along the imaging direction.

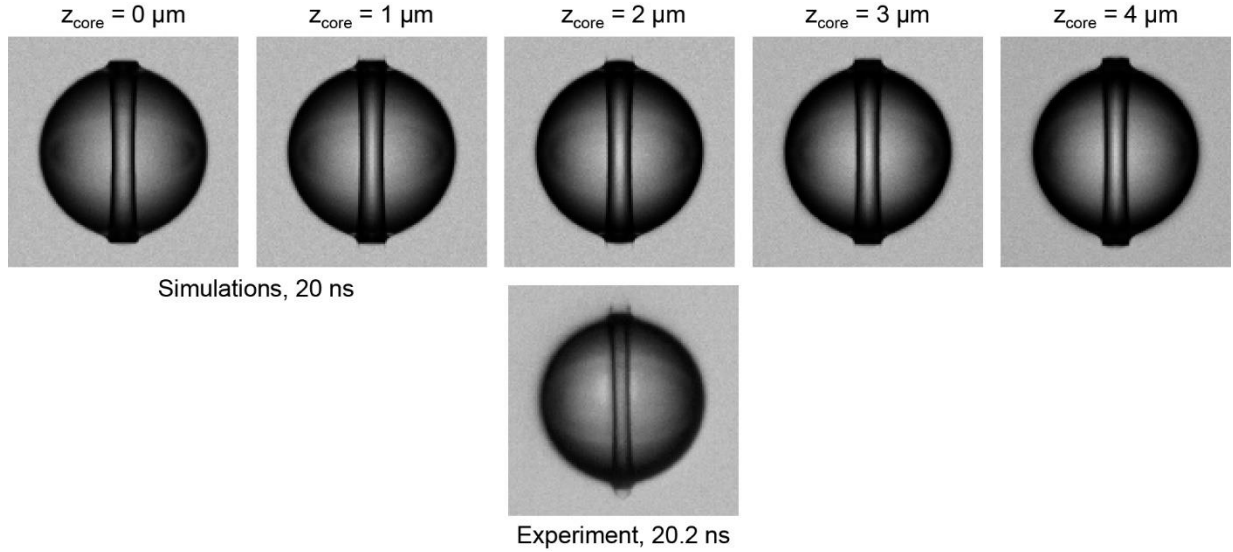

**Figure S9.** Determination of the misalignment between the drop and X rays. The experimental image of a negative image is compared to simulations made for a range of misalignments. The aspect ratio of the negative pressure wave is best replicated at 2  $\mu\text{m}$ , with a precision of 1  $\mu\text{m}$ .

#### 6.4. Refinement of CFD model for the ablation experiment without core formation

In the initial simulations of the weak ablation case without hole formation, we observed a relatively low amplitude pressure wave emerging from the regions where the X-ray pulse intersected the surface of the drop. A plot of the corresponding pressure distribution is shown in Figure S10. Since the amplitude of this extra pressure wave is smaller than the shock and its reflection, which are barely visible in the experiment, it cannot be determined from CFD if the extra wave would be visible in experiments (and thus real). However, according to the simulated image shown in Fig. S10, the low amplitude wave would generate features in the simulated image that were not seen in the experiment. Therefore, this wave either does not exist in the experiment, or it has a lower amplitude. We note that in Fig. S10, we used a higher filament pressure (275 MPa) than the best-matched pressure (195 MPa) used for Supplementary Movie 4, because the unphysical wave is difficult to see in single frames.

The low amplitude wave is a rarefaction wave that appeared in the CFD simulations because the parts of the X-ray heated filament near the drop surface expanded into free space faster than the rest of the filament, which was restricted by the surrounding liquid. In the original version of the CFD model, the expansion towards free space was unconstrained, and this generated the wave. However, since the filament is hot, its ends will evaporate. Evaporation leads to a reactive force and to an associated reactive pressure, which is equal to the vapor pressure [27]. This reactive pressure will restrict the expansion of the filament. Based on the energy of the X-ray pulse, we estimated that the filament becomes superheated, which leads to high vapor pressures, possibly all the way up to the critical pressure of 22 MPa.

To suppress the unphysical wave in simulations, we extended the CFD model with a modified interface condition. By default, at the interface between water and air, we solved a two-phase Riemann problem to obtain the velocity of the interface as well as the numerical evolution terms for both phases [25]. The reactive pressure due to evaporation is missing from our model and thus also missing in the Riemann

problem, but as discussed above, we expect the interface movement at the ends of the filament to be close to zero. Therefore, we added an additional interface Riemann problem that constrains the interface velocity to zero and computes the remaining states accordingly. To avoid abrupt changes in the interface conditions, we blended between the constrained Riemann problem and the standard Riemann problem with a Gaussian profile,  $\exp(-2/(x/5 \mu\text{m})^2)$ , where  $x$  is the distance from the drop axis.

The results of the updated, “velocity-capped” CFD simulation no longer displayed the wave, and the wave was no longer visible in the image simulations, as shown in Fig. S10. A rarefaction region caused by the oblique reflection of the shock wave still can be observed the pressure distribution, but it has a much lower amplitude than the unphysical wave. The simulated frames from Supplementary Movie 4 were calculated using the velocity-capped CFD model.

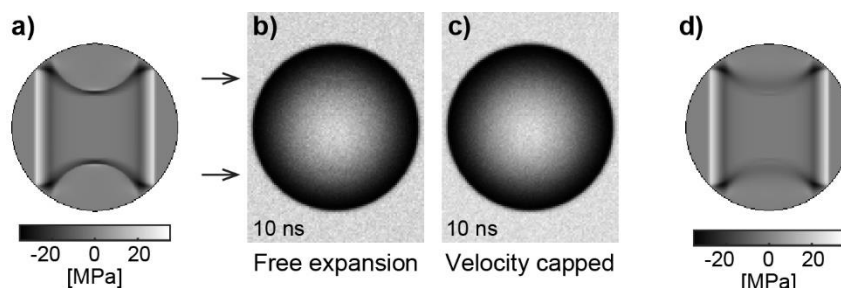

**Figure S10.** Refinement of the CFD model using image simulations. (a) Pressure distribution from an initial CFD model, and (b) corresponding simulated image, both displaying a pressure wave that is not observed in the experimental image. The arrows indicate the height of the wave features. (c,d) Corresponding results from a “velocity-capped” CFD model that restricts the expansion of the filament into the surrounding gas, to account for the reactive pressure due to evaporation. The differences between images may only be visible on a computer screen.

## 7. Supplementary movies

Table ST1 lists the supplementary movies and their composition. Supplementary Movies 1-3 display the dynamics of droplet merging, for two imaging conditions: the default setup where the droplets remained in focus while merging, and a tilted-jet setup in which the droplets travelled across the object plane while merging. In both cases, the experimental frames were cropped such that the droplet appears centered in the rendered images. In the experiments, the droplets travelled downwards while merging, and this can be observed in the Supplementary Movie 1 as a dark spot in the background. The spot was stationary in the experiment, but appears to travel upwards in the processed movie.

Supplementary Movie 1 shows experimental and simulated images for the experiment where the drops remained in focus. Supplementary Movies 2 and 3 show experimental and simulated images for merging drops that travelled across the focal plane, with the simulated drops making angles of  $4^\circ$  and  $5^\circ$ , respectively, to the image plane. As explained in Section 6.2., the merging drop rotated, thus the experimental frames at short time delays are best matched in Supplementary Movie 3 ( $5^\circ$ ), while the frames at the long time delays are best matched in Supplementary Movie 2 ( $4^\circ$ ).

Supplementary Movie 4 shows experimental and simulated images for the weak ablation experiment. Both the outgoing pressure wave and the reflected wave are replicated in the simulated movie, despite being barely visible. The frames show images with delays increasing in 1 ns time steps, except from 10 ns to 18 ns where the delays increased in 4 ns steps. Since the drop magnifies the image of the interior of the drop, from approximately 10 to 18 ns the waves are near the edge of the drop and not visible in the images. The

frames were matched based on their visual appearance, and the time delays for the experiment are approximately 1 ns higher than for the simulation across the entire movie, which could be explained by an experimental error in determining the exact time of arrival of the X-ray pulse.

Supplementary Movie 5 shows experimental and simulated images for the strong ablation experiment. The frames were chosen at time delays increasing in 1 ns steps except for the 10 ns to 18 ns interval, same as in Supplementary Movie 4. In the experiment the drops were misaligned from the X ray beam by 2  $\mu\text{m}$  on average, and the simulations replicated this misalignment (see Section 6.3.). Some of the frames, for example the one at 24 ns, were misaligned by a different amount, and the match between simulation and experiment is of lower quality. The simulated images of the negative pressure reflection, although not identical to the experiment, replicate the brighter-and-darker patterns observed experimentally.

**Table ST1.** Supplementary movies.

| Nr. | File name      | Description                                                                                           | Composition (left to right)                                    |
|-----|----------------|-------------------------------------------------------------------------------------------------------|----------------------------------------------------------------|
| 1   | SuppMovie1.avi | Merging of 3 drops travelling in the object plane (in focus)                                          | Experimental image<br>2D>3D ray tracing<br>CFD and ray tracing |
| 2   | SuppMovie2.avi | Merging of 3 drops travelling through the object plane (out of focus), simulated drops at a 4° angle. | Experimental image<br>2D>3D ray tracing<br>CFD and ray tracing |
| 3   | SuppMovie3.avi | Merging of 3 drops travelling through the object plane (out of focus), simulated drops at a 5° angle. | Experimental image<br>2D>3D ray tracing<br>CFD and ray tracing |
| 4   | SuppMovie4.avi | Drop ablated by X-ray pulse, below the threshold for cavity formation                                 | Experimental image<br>CFD and ray tracing                      |
| 5   | SuppMovie5.avi | Drop ablated by X-ray pulse, above the threshold for cavity formation                                 | Experimental image<br>CFD and ray tracing                      |

## 8. Image processing

The images shown in this study, including the frames shown in the supplementary movies, were rendered on a linear intensity scale and preserve the original pixel resolution. The experimental movies were recorded using the camera software (Phantom PCC v3.0) in a packed 10-bit cine format, then exported as 8-bit monochrome uncompressed .avi files. Before exporting, the movies were set to a linear gain profile ( $\gamma = 1$ ) and the linear gain was adjusted such that the background of the images was at approximately three quarters of the image saturation level, which is 255 for an 8-bit movie.

The raw simulated images are matrices that contain the number of ray hits in each pixel. The ray hits were scaled such that the background of simulated images had the same relative intensity as the experimental images (three quarters of the 8-bit saturation level), generating 8-bit grayscale images that were used in the figures and the movies.

All the images and movies were processed and annotated using MATLAB, version R2023b or later. The movies were saved from MATLAB using the “Grayscale AVI” profile, which produces an uncompressed AVI file with 8-bit grayscale video.

## 9. References

### *References present in the main text*

- [13] M. Liang, *et al.*, *The Coherent X-ray Imaging instrument at the Linac Coherent Light Source*, J. Synchrotron Radiat., **22**, 514 (2015). <https://doi.org/10.1107/s160057751500449x>
- [14] M. Levoy, P. Hanrahan, *Light field rendering*, in: M.C. Whitton (Ed.) *Seminal Graphics Papers: Pushing the Boundaries*, ACM, USA, 2023, pp. 441. <https://doi.org/10.1145/3596711>
- [15] N.A. Adams, *et al.*, *ALPACA - Adaptive Level-set PARallel Code Alpaca*, Technical University of Munich, Garching, Germany (2022). <https://doi.org/10.14459/2022mp1647482>
- [16] C.A. Stan, *et al.*, *Negative Pressures and Spallation in Water Drops Subjected to Nanosecond Shock Waves*, J. Phys. Chem. Lett., **7**, 2055 (2016). <https://doi.org/10.1021/acs.jpclett.6b00687>
- [17] P. Emma, *et al.*, *First lasing and operation of an angstrom-wavelength free-electron laser*, Nat. Photon., **4**, 641 (2010). <https://doi.org/10.1038/nphoton.2010.176>
- [18] T. Paula, S. Adami, N.A. Adams, *Analysis of the early stages of liquid-water-drop explosion by numerical simulation*, Phys. Rev. Fluids, **4**, 044003 (2019). <https://doi.org/10.1103/PhysRevFluids.4.044003>
- [19] C.A. Stan, *et al.*, *The Magnitude and Waveform of Shock Waves Induced by X-ray Lasers in Water*, Appl. Sci.-Basel, **10**, 1497 (2020). <https://doi.org/10.3390/app10041497>
- [20] O. Le Métayer, R. Saurel, *The Noble-Abel Stiffened-Gas equation of state*, Phys. Fluids, **28**, 046102 (2016). <https://doi.org/10.1063/1.4945981>
- [21] W. Wagner, A. Pruß, *The IAPWS formulation 1995 for the thermodynamic properties of ordinary water substance for general and scientific use*, J. Phys. Chem. Ref. Data, **31**, 387 (2002). <https://doi.org/10.1063/1.1461829>
- [22] A.H. Harvey, J.S. Gallagher, J. Sengers, *Revised formulation for the refractive index of water and steam as a function of wavelength, temperature and density*, J. Phys. Chem. Ref. Data, **27**, 761 (1998). <https://doi.org/10.1063/1.556029>

### *References unique to the Supplemental Material*

- [23] A. Kalita, *et al.*, *Microstructure and crystal order during freezing of supercooled water drops*, Nature, **620**, 557 (2023). <https://doi.org/10.1038/s41586-023-06283-2>
- [24] C.A. Stan, A. Kalita, M. Mrozek-McCourt, *Modeling of supercooling, solidification, and freezing stages of water drops*, Zenodo (2023). <https://doi.org/10.5281/zenodo.7908647>
- [25] T. Paula, S. Adami, N.A. Adams, *A robust high-resolution discrete-equations method for compressible multi-phase flow with accurate interface capturing*, J. Comput. Phys., **491**, 112371 (2023). <https://doi.org/10.1016/j.jcp.2023.112371>
- [26] N. Vargaftik, B.N. Volkov, L. Voljak, *International tables of the surface tension of water*, J. Phys. Chem. Ref. Data, **12**, 817 (1983). <https://doi.org/10.1063/1.555688>
- [27] C.A. Stan, A. Kalita, S. Marte, T.F. Kaldawi, P.R. Willmott, S. Boutet, *Rocket drops: The self-propulsion of supercooled freezing drops*, Phys. Rev. Fluids, **8**, L021601 (2023). <https://doi.org/10.1103/PhysRevFluids.8.L021601>
